# Supplementary material for: A Point-Based Approach to Efficient LiDAR Multi-Task Perception
Source: arXiv:2404.12798 source file (2024-04-19)
Supplement: Supplementary file 1 [file X_suppl.tex]

\clearpage
\setcounter{page}{1}
\maketitlesupplementary

\section{Rationale}
\label{sec:rationale}
Having the supplementary compiled together with the main paper means that:
\begin{itemize}
\item The supplementary can back-reference sections of the main paper, for example, we can refer to \cref{sec:intro};
\item The main paper can forward reference sub-sections within the supplementary explicitly (e.g. referring to a particular experiment); 
\item When submitted to arXiv, the supplementary will already be included at the end of the paper.
\end{itemize}

\section{Connectivity analysis}

In the proposed point-centric attention operation, the field of view is determined by the local window size, which is also referred to as the neighborhood size. In this section, we analyze the impact of the neighborhood size on the field of view for different data distributions. To achieve this, we conduct a connectivity analysis that assesses the number of transformer layers required for a point feature to reach all other points in the current scan, as shown in Figure \ref{fig:connectivity_analysis}. Since the ball query used in constructing local attention windows is non-deterministic and testing all points in the point cloud for the entire dataset is not feasible, and the connectivity varies with the scene composition, we report statistical values obtained by sampling 20 points per scan for each frame in the respective dataset.
The results are summarized in \tabref{}.
